# Supplementary material for: Unbalanced Optimal Transport: A Unified Framework for Object Detection
Source: arXiv:2307.02402 source file (2023-07-05)
Supplement: Supplementary file 1 [file code.tex]

\section{Code}
We plan to make our code available. This section will provide a discussion of it.
